# Supplementary material for: Effect of Notch Structure on Magnetic Domain Movement in Planar Nanowires
Source: arXiv:1711.08788 source file (2017-11-23)
Supplement: Supplementary file 1 [file Supplementary_Information.pdf]

# Supplementary Information for " Effect of Notch Structure on Magnetic Domain Movement in Planar Nanowires "

Hua Ling,[1, 2, a)] Junlin Wang,[1, 2, a)] Xianyang Lu,[3, 2] Junran Zhang,[2] Li Chen,[4] Christopher Reardon,[3] Jason Zhang,[3] Yichuan Wang,[3, 2] Yu Yan,[1, 2] Jing Wu,[3, 2, b)] and Yongbing Xu[1, 2, c)]

[1]Spintronics and Nanodevice laboratory, Department of Electronic Engineering, University of York, York YO10 5DD,United Kingdom

[2]York-Nanjing International Center of Spintronics (YNICS), School of Electronic Science and Engineering, Nanjing University, Nanjing 210093, China

[3]Department of Physics, University of York, York YO10 5DD, United Kingdom

[4]Faculty of Engineering, University of Leeds, Woodhouse Lane, Leeds LS2 9JT, United Kingdom

E-mail: jing.wu@york.ac.uk and yongbing.xu@york.ac.uk

# 1. The Hysteresis loops of 600 nm depth notch

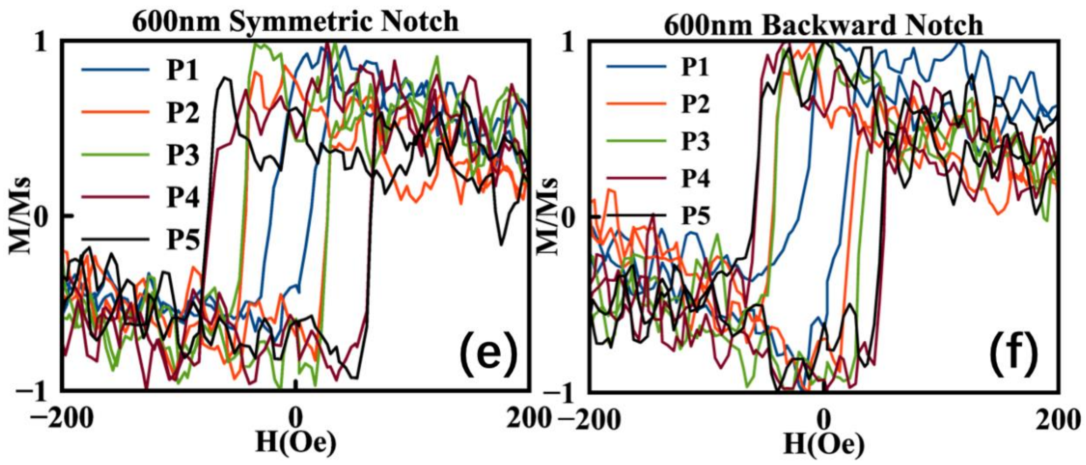


Fig. S1 (a) The Hysteresis loops of 600 nm depth symmetric notch configuration. (b) Hysteresis loops of 600 nm depth backward notch configuration. The P1-P5 is defined in the manuscript. The nanowire with 600 nm depth backward notch has the smallest depinning magnetic field in the nanowires with 600 nm depth notch. The difference between each point in the nanowires with 600 nm depth notch is larger than in the nanowire with 400 nm depth notch.

The hysteresis loops in Fig. S1 (a) is for 600 nm symmetric notch configuration. The coercivity of the position 1 to position 5 are about 18 Oe, 35 Oe, 35 Oe, 69 Oe and 69 Oe, respectively. Firstly, the domain nucleated on the pad at 10 Oe and started propagated to the wire at -40 Oe, then pinned at the notch before -67 Oe. After the external field larger than -87 Oe the full wire had been saturated along the negative direction. When the external field decreases to -5 Oe, the domains started to nucleate at the pad and started propagated to the wire at 17 Oe, the depinning field is 61 Oe. Finally, the full wire was saturated along the positive direction at 74 Oe. The jump is not clearly shown by the hysteresis loops. The hysteresis loops in Fig. S1 (b) is for 600 nm backward notch configuration. The coercivity of the position 1 to position 5 are about 15 Oe, 32.5 Oe, 36.5 Oe, 53.5 Oe and 53.5 Oe, respectively. Firstly, the domain nucleated on the pad at 0 Oe and started propagated to the wire at -35 Oe, then pinned at the notch before -53 Oe. after -83 Oe the full wire had been saturated along the negative direction. When the minimum external field approach, the applied field increased. At 0 Oe, the domains started to nucleate at the pad and started propagated to the wire at 30 Oe, the depinning field is 43 Oe. Finally, the full wire was saturated along the positive direction at 51 Oe. The jump is not clearly shown by the hysteresis loops.

## 2. The domain configuration of 600 nm depth notch

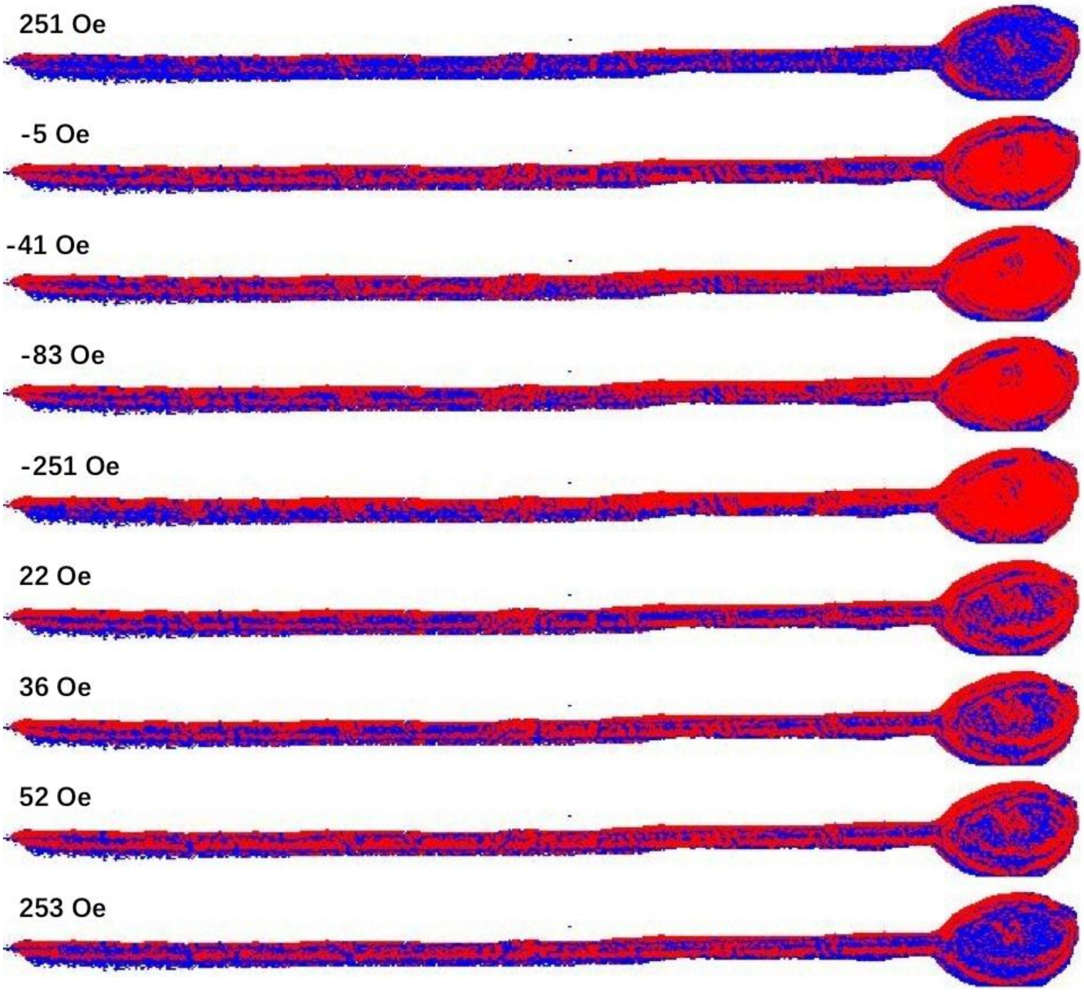


Fig. S2 Kerr image contrast images for 600 nm forward notch depth nanowire. The positive external field direction is to the right.

The contrast images of Fig. S3 demonstrating the DWs pinning and depinning in 400 nm symmetric notch depth nanowire. When the external field equal to 251 Oe, -251 Oe and 253 Oe external field, the images are almost blue or red, this is means the nanowire is the saturation state. When the external field reduced to negative, the domains first nucleated at the pad. At -5 Oe, a typical contrast images of pad nucleation can be clearly observed and the DWs pined at the wire. When the external field equal -41 Oe, the domains broken though the DWs on the wire and pined at the notch as known as notch pinning state. In the negative side of the hysteresis loop, the notch depinning state and double domains phenomenon displays at -83 Oe, compare to the saturation state image at -251 Oe the red line after the notch is narrower. With the reductions of negative applied field, the positive domains

nucleate. The positive domains first can be seen at the pad and the many blue pixels appeared when the external field was 22 Oe and the notch pinning state displays at 36 Oe. The contrast image of notch depinning state appeared when external field is 52 Oe.

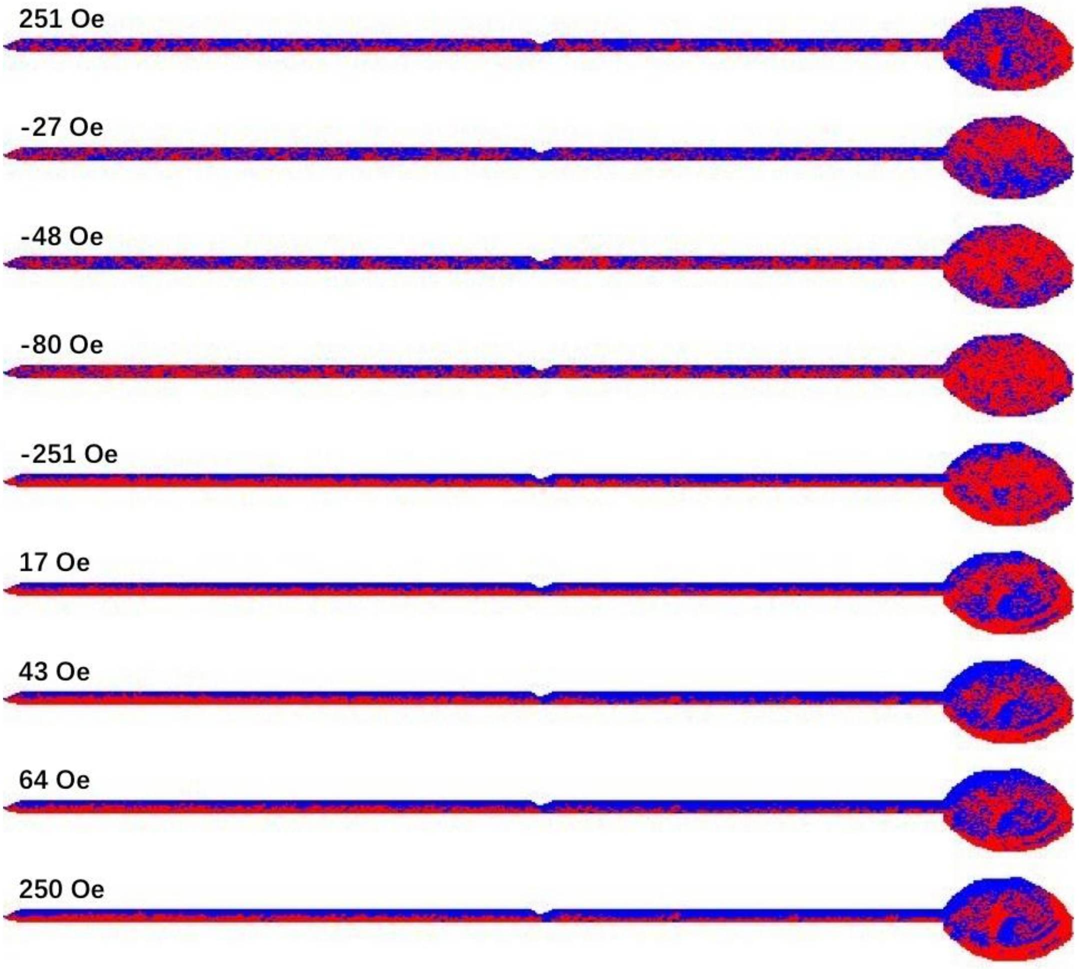


Fig. S3 Kerr image contrast images for 600 nm symmetric notch depth nanowire. The positive external field direction is to the right.

The contrast images of Fig. S3 demonstrates the DWs pinning and depinning in 400 nm symmetric notch depth nanowire. When the magnetic applied field equal to 251 Oe, -251 Oe and 250 Oe, the images are almost blue or red, this is the saturation state. When the external field reduced to negative, the domains first nucleated at the pad of the nanowire. A typical contrast images of pad nucleation can be clearly observed in Fig. S3 and the DWs are pined at the wire when the external field is -27 Oe. At -48 Oe, the domains broken though the DWs on the wire and pined at the notch as known as notch pinning state. In the negative side of the hysteresis loop, the notch depinning state and double

domains phenomenon can be seen at -80 Oe, the red line after the notch is narrower compare to the saturation state image at -251 Oe. With the reductions of negative applied field, the positive domains nucleate. The positive domains first can be seen at the pad and the many blue pixels appeared when the external field was 17 Oe and the notch pinning state displays at 43 Oe. The contrast image of notch depinning state appeared when external field is 64 Oe.

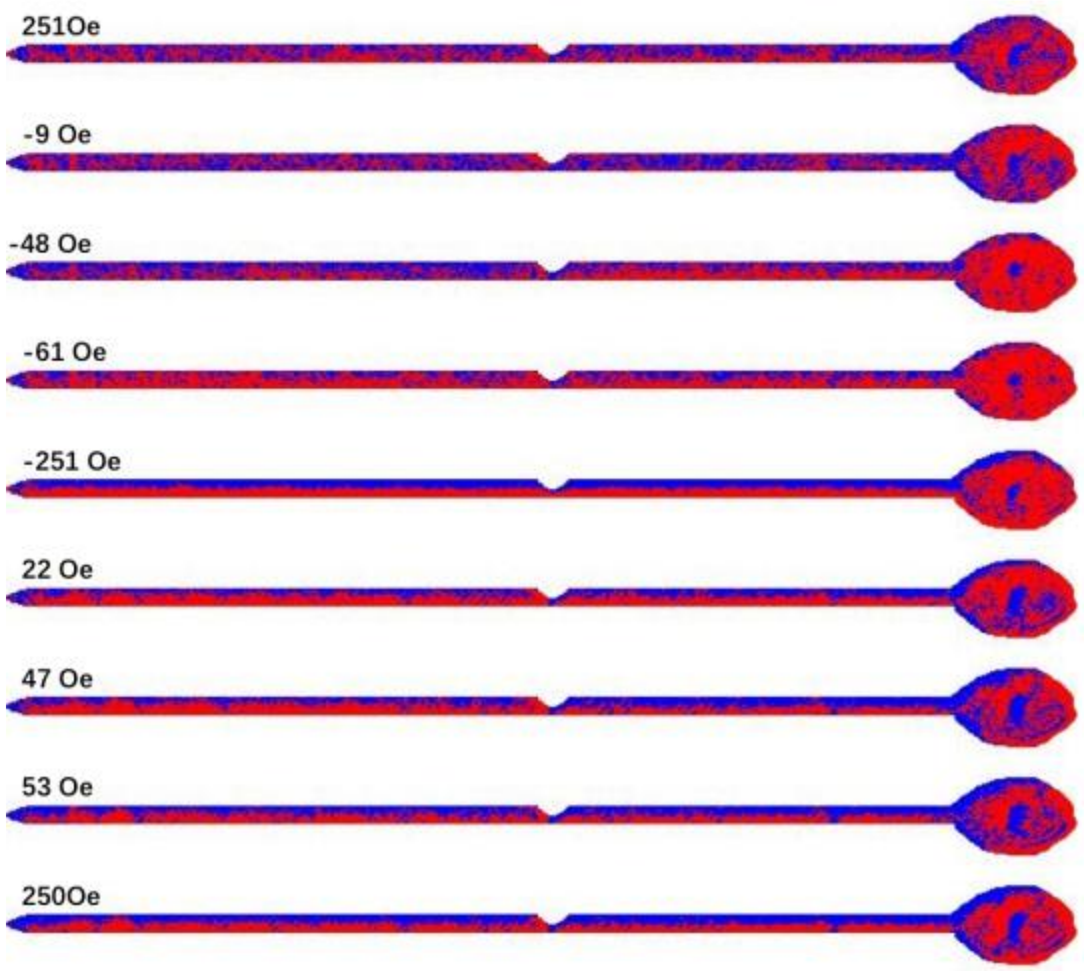


Fig. S4 Kerr image contrast images for 600 nm backward notch depth nanowire. The positive external field direction is to the right.

The contrast images of Fig. S4 demonstrates the DWs pinning and depinning in 400 nm symmetric notch depth nanowire. When the magnetic applied field equal to 251 Oe, -251 Oe and 251 Oe, the images are almost blue or red, this is the saturation state. When the external field reduced to negative, the domains first nucleated at the pad of the nanowire. A typical contrast images of pad nucleation can be clearly observed in Fig. S4 and the DWs are pined at the wire when the external field is -9 Oe. At -

48 Oe, the domains broken though the DWs on the wire and pined at the notch as known as notch pinning state. In the negative side of the hysteresis loop, the notch depinning state and double domains phenomenon can be seen at -61 Oe, the red line after the notch is narrower compare to the saturation state image at -251 Oe. With the reductions of negative applied field, the positive domains nucleate. The positive domains first can be seen at the pad and the many blue pixels appeared when the external field was 22 Oe and the notch pinning state displays at 47 Oe. The contrast image of notch depinning state appeared when external field is 53 Oe.
